# Supplementary material for: Reconnecting the Estranged Relationships: Optimizing the Influence Propagation in Evolving Networks
Source: arXiv:2205.05236 source file (2022-05-11)
Supplement: Supplementary file 1 [file Appendix.tex]

\iffalse
\begin{algorithm}[t!]
    \caption{Build UF$(G_t)$}
\label{alg:index-based}
	\KwIn{$\mathcal{G}=\{G_i\}^{t-1}_1:$ an evolving graph, $G_t:$ the predicted snapshot graph, and $\mathcal{U}$: a group of users}
	\KwOut{ $UF(G_t)$ the Union Find index} 
	\BlankLine

\SetKwFunction{FMain}{MC-Estimate}
    \SetKwProg{Fn}{Function}{:}{}
    \Fn{\FMain{$\mathcal{U},e$}}{
    $count \leftarrow 0$, $G'\leftarrow \widehat{G} \oplus e$; \\
    \For{$j = 1$ to $R$}{
       Simulate diffusion process on graph $G'$ start from seed set $\mathcal{U}$; \\
       $n_a\leftarrow$ the number of activated nodes; \\ % after the diffusion ends; \\
       $count \leftarrow count + n_a$; \\
    }
   \Return{$count / R$}
}

\SetKwFunction{FMain}{MC-Estimate}
    \SetKwProg{Fn}{Function}{:}{}
    \Fn{\FMain{$\mathcal{U},e$}}{
    $count \leftarrow 0$, $G'\leftarrow \widehat{G} \oplus e$; \\
    \For{$j = 1$ to $R$}{
       Simulate diffusion process on graph $G'$ start from seed set $\mathcal{U}$; \\
       $n_a\leftarrow$ the number of activated nodes; \\ % after the diffusion ends; \\
       $count \leftarrow count + n_a$; \\
    }
   \Return{$count / R$}
}

\SetKwFunction{FMain}{MC-Estimate}
    \SetKwProg{Fn}{Function}{:}{}
    \Fn{\FMain{$\mathcal{U},e$}}{
    $count \leftarrow 0$, $G'\leftarrow \widehat{G} \oplus e$; \\
    \For{$j = 1$ to $R$}{
       Simulate diffusion process on graph $G'$ start from seed set $\mathcal{U}$; \\
       $n_a\leftarrow$ the number of activated nodes; \\ % after the diffusion ends; \\
       $count \leftarrow count + n_a$; \\
    }
   \Return{$count / R$}
}
	
\Return{$UF(G_t)$}
\end{algorithm}
\fi

\iffalse
\begin{algorithm}[t!] %[hbt!] 
	\caption{\textbf{RT$l$L:} Order-based SBG} % $(G_t, l, \mathcal{U}, CE)$}}
%	\caption{\textit{Sketch-Estimate Algorithm}}
	\label{alg:basic1}
	\KwIn{$G_t:$ the predicted graph, $l$: the number of selected edges, $\mathcal{U}$: a group of users, and $\mathcal{L}$: Labeling scheme}
	\KwOut{ $\widehat{S}:$ the optimal Reconnecting edge set} 
	\BlankLine

	Initialize $\widehat{S}\leftarrow \emptyset$, $\widehat{G}\leftarrow G_t$; Priority queue $Q \leftarrow \emptyset$ \\ % $t\leftarrow 1$; \\ 
%	Candidate edges set $CE\in \{\mathcal{G}\setminus G_t\}$ \\
    $\widehat{CE}\leftarrow$ Reducing CE \# BFS $($CE$, \mathcal{U})$; /*using Algorithm~\ref{alg:BFS_prunning_edges} */ \\
	\For {each edge $e=(u,v)\in \widehat{CE}$}{ 
        add $(v, L(v))$ into $Q$; \\
    }

	\For {$i = 1$ to $l$}{ 
%	/* Candidate edges $e\in \{\mathcal{G}\setminus G_t\}$ */ \\
	    $\widehat{e} \leftarrow \mathop{\arg\max}_{e\in CE}$ Sketch-Estimate$(\mathcal{U},e)$; \\
        $\widehat{S}\leftarrow \widehat{S}\cup \widehat{e}$, $\widehat{G}\leftarrow \widehat{G} \oplus \widehat{e}$
    }

\SetKwFunction{FMain}{Sketch-Estimate}
    \SetKwProg{Fn}{Function}{:}{}
    \Fn{\FMain{$\mathcal{U},e$}}{
    $count \leftarrow 0$, $count_R \leftarrow 0$, $G'\leftarrow \widehat{G} \oplus e$;  \\
    \For{$j = 1$ to $R$}{
       $n_R\leftarrow$ the number of reached nodes from $v$; \\
       $n_a\leftarrow$ the size of reached nodes from $v$ while eliminate the nodes that reached by $\mathcal{U\cup \widehat{S}}$ in $G^j_{sg}$; \\ % after the diffusion ends; \\
       $count \leftarrow count + n_a$; \\
       $count_R \leftarrow count_R + n_R$; \\
    }
    update $L(v) = (v, count_R)$ from $\mathcal{L}$; \\
   \Return{$count / R$}
}
\textbf{End Function}

\Return{$\widehat{S}$}	
\end{algorithm}

\begin{algorithm}[t!] %[hbt!] 
	\caption{\textit{Generate $\#$ Labeling Construction}}
%	\caption{\textit{Order-based RT$l$L$(G_t, l, \mathcal{U}, CE)$}}
	\label{alg:basic1}
%	\KwIn{$\mathcal{G}=\{G_i\}^{t-1}_1:$ an evolving graph}
%	\KwOut{ $\mathcal{L}:$ Labeling, and $G_{sg}: $ Sampling subgraph sketch} 
	\BlankLine
	Predict the snapshot graph $G_t$ from $\mathcal{G}$~\cite{zhang2018link} \\
	Candidate edges set $CE\in \{\mathcal{G}\setminus G_t\}$ \\
%	Initialize $\widehat{S}\leftarrow \emptyset$, $G_{sg}\leftarrow \emptyset$; labeling scheme $\mathcal{L} \leftarrow \emptyset$; \\
	Initialize the sampling subgraph sketch $G_{sg}\leftarrow \emptyset$; labeling scheme $\mathcal{L} \leftarrow \emptyset$; \\
%	Candidate edges set $CE\in \{\mathcal{G}\setminus G_t\}$ \\
    \For {$i = 1$ to $R$}{
        $G^i_{sg} \leftarrow (V^i_{sg} = \emptyset, E^i_{sg} = \emptyset)$; \\
        generate sampling subgraph $G^i_t$ to update $G^i_{sg}$ \\
        add $G^i_{sg}$ into $G_{sg}$ \\
    }
	\For {each edge $e=(u,v)\in CE$}{ 
        $\sigma(v)\leftarrow$ the number of vertices that can be reached from $v$ in $G_t$; \\
        $L(v)\leftarrow (v, \sigma(v))$; \\
        add $L(v)$ into $\mathcal{L}$; \\
    }
\Return{$\mathcal{L}, G_{sg}$}	
\end{algorithm}
\fi


\iffalse
\begin{algorithm}[t!] %[hbt!] 
	\caption{\textbf{RT$l$L:} Order-based SBG} % $(G_t, l, \mathcal{U}, CE)$}}
	\label{alg:basic1}
	\KwIn{$G_t:$ the predicted graph, $l$: the number of selected edges, $\mathcal{U}$: a group of users, $CE$: candidate edges, and ($\mathcal{L}$, $G_{sg}$): Labeling scheme}
	\KwOut{ $\widehat{S}:$ the optimal Reconnecting edge set} 
	\BlankLine

	Initialize $\widehat{S}\leftarrow \emptyset$, Priority queue $Q$, and Array $SG[\theta_2][|V|]$; \\ % $t\leftarrow 1$; \\ 
    $\widehat{CE}\leftarrow$ Reducing CE \# BFS $($CE$, \mathcal{U})$; /*using Algorithm~\ref{alg:BFS_prunning_edges} */ \\
	\For {each edge $e=(u,v)\in \widehat{CE}$}{ 
	    $q.e \leftarrow \mathcal{L}.{L(e)}$; \\
        add $(e, q.e)$ into $Q$; \\
    }
    \For {$i = 1$ to $\theta_2$}{ 
         \For{each $u \leftsquigarrow \mathcal{U}$ in $G_t$}{
               $SG[i][u]\leftarrow 1$; \\
         }
    }

	\For {$j = 1$ to $l$}{ 
%	/* Candidate edges $e\in \{\mathcal{G}\setminus G_t\}$ */ \\
%	    $e' \leftarrow \mathop{\arg\max}_{e\in CE}$ Sketch-Estimate$(\mathcal{U},e)$; \\
	    $(e',q.{e'}) \leftarrow Q.front$ ; \\
	    $I_{max} \leftarrow 0$; $\widehat{e} \leftarrow e'$; \\
%	    $\widehat{G_{sg}^j} \leftarrow G_{sg}^j \oplus \widehat{S}$; \\
	    \While{$I_{max} < q.{e'}$}{
	          $I_{max} \leftarrow$ Sketch-Estimate$(\mathcal{U}, \widehat{e})$; \\
	          $\widehat{e} \leftarrow e'$; 
	          $(e',q.{e'}) \leftarrow Q.front$ ; \\
	    }
        $\widehat{S}\leftarrow \widehat{S}\cup \widehat{e}=(\widehat{u},\widehat{v})$;\\ %, $\widehat{G}\leftarrow \widehat{G} \oplus \widehat{e}$
        \For{$m = 1$ to $\theta_2$}{
            \If{$SG[m][\widehat{u}]==1$ $\&\&$ $SG[m][\widehat{v}]==0$}{
            $SG[m][\widehat{v}]\leftarrow 1$; \\
            \For{each $u' \leftsquigarrow \widehat{e}$ in $G^m_{sg}$}{
                $SG[m][u]\leftarrow 1$; \\
            }
            }
        }
    }

\SetKwFunction{FMain}{Sketch-Estimate}
    \SetKwProg{Fn}{Function}{:}{}
    \Fn{\FMain{$\mathcal{U},e = (u,v)$}}{
    $count \leftarrow 0$, $count_R \leftarrow 0$, $G'\leftarrow \widehat{G} \oplus e$;  \\
    \For{$k = 1$ to $\theta_2$}{
%        \If{$\{Array[k][u] \wedge Array[k][v]\} \vee \neg\{Array[k][u] \wedge Array[k][v]\} $}{

         \While{$SG[k][u]==1$ $\&\&$ $SG[k][v]==0$}{
       $n_a\leftarrow$ the size of reached nodes $u'$ from $e$ with $SG[k][u']==0$; \\ % while eliminate the nodes that reached by $\mathcal{U\cup \widehat{S}}$ in $\widehat{G^k_{sg}}$; \\ % after the diffusion ends; \\
       $count \leftarrow count + n_a$; \\
       }

       \If{$flag(e) == 0$}{
            $n_R\leftarrow$ the number of reached nodes from $e$ in $G^k_{sg}$; \\
       }
%       \Else{
%            Continue; \\
%       }
    }
    update $(e, q.e) \leftarrow (e, count / R)$ of $Q$; \\
    \If{$flag(e) == 0$}{
       $count_R \leftarrow count_R + n_R$; $flag(e)\leftarrow 1$;\\
       update $(L(e),flag(e))\leftarrow  (count_R / R, 1)$ of $\mathcal{L}$; \\
    }
   \Return{$count / R$}
}
\textbf{End Function}

\Return{$\widehat{S}$}	
\end{algorithm}
\fi
